# Supplementary material for: Language Evolution with Deep Learning
Source: arXiv:2403.11958 source file (2024-03-18)
Supplement: Supplementary file 1 [file appendix.tex]

\section{Formalizing Lewis Games as a machine learning problem}
\label{subsec:formalism_game}

% Idéalement il faudrait passer en 3 paragraphes:
% 1. Markov Game
% 2. Policies
% 3. Optim pb
% Pour qu'ensuite il y ait un echo dans toutes les parties suivantes
Toward using machine learning tools, it is crucial to rigorously identify the key modelling elements of the communication game, and to define a unified set of notations. To this extend, we here use the Markov Games' framework~\citep{littman1994markov}, which is the classic mathematical framework for interactive game learning, and is the basis of the reinforcement learning tools that we will introduce. 
% From it, we surface out three main modelling elements that should be designed to implement a communication game: the game, the agents, and the optimization problem.

\paragraph{The game}
%We first aim at framing Lewis Games as Markov Games. To ease comprehension, we will use the case of the Visual Discrimination Game as a thread example (see Table~\ref{tab:taxo_tasks}). %In this game, the sender in observing an image. It then communicates a message to the receiver, that has to recover this original image among a set of $N$ images.
Following Markov Games formalism, Lewis Games can be subdivided into five core elements: the states, the actions of the sender, the actions of the receiver, the game dynamics, and the game reward. It is  written as a tuple as follow:
\begin{align*}      (\mathcal{S},\mathcal{A}_{\sender},\mathcal{A}_{\receiver},\mathcal{P},\mathcal{R})
\end{align*}

when detailed, corresponds to: 
\begin{itemize}
    \item $\mathcal{S}$ is a set of states. It describes all the possible configurations of the game at one instant. Besides, each agent may only observe a snapshot of this state, which is described by the two observations $o_{\sender}$ and $o_{\receiver}$. 
    %example
    In the Visual Discrimination Game, the sender observation is an image and the receiver observation is both the set of images (correct image and distractors) and the message sent by the sender.
    \item $\mathcal{A}_{\sender}$ and $\mathcal{A}_{\receiver}$ are the set of actions for the sender and the receiver. In the context of Lewis Games, sender's actions $\mathcal{A}_{\sender}$ are the messages the sender can send and receiver's actions $\mathcal{A}_{\receiver}$ depends on the task. %To ease reading, we will next denote $\mathcal{A}_{sender}$ by $\mathcal{M}$ and a message sent by the sender $m$. 
    %Note that Lewis Games are turn-based Markov Games, meaning that the two agents always act one after the other.
    %example
    In the Visual Discrimination Game, the set of sender actions $\mathcal{A}_{\sender}$ is the set of messages the sender can send to the receiver ; actions of the receiver $\mathcal{A}_{\receiver}$ are the different choices of images when trying to retrieve the image seen by the sender.
    %
    %\item $\mathcal{O}_{sender}$ and $\mathcal{O}_{receiver}$ are the functions that map all the information available in the environment to observations of the two agents $\mathcal{o}_{sender}$ and $o_{receiver}$. It can be either the states, partial view of the states or the actions of the other agents. %example
    %In the Visual Discrimination Game, the state $\mathcal{s}$ is the set of $N$ images, $o_{sender}$ is a random image among those $N$ images and $o_{receiver}$ is both full observation of the state $s$ and the action of the sender, i.e the message sent.
    %
    \item $\mathcal{P}:(\mathcal{S}\times\mathcal{A}_{\sender}\times\mathcal{A}_{\receiver},\mathcal{S}) \to [0,1]$ is the probability of reaching state $s' \in \mathcal{S}$ when agents perform actions $a_{\sender} \in \mathcal{A}_{\sender}$ and $a_{\receiver} \in \mathcal{A}_{\receiver}$ while being in the state $s \in \mathcal{S}$. 
    %example
    In the Visual Discrimination Game, the probability $\mathcal{P}$ is uniform and thus does not take any role. $\mathcal{P}$ is useful when modeling a complex environment that depends on agents' actions.
    \item $\mathcal{R}:(\mathcal{S},\mathcal{A}_{\sender},\mathcal{A}_{\receiver}) \to \mathbb{R}$ is a reward function that returns a common pay-off for the two agents when the agents perform actions $a_{\sender} \in \mathcal{A}_{\sender}$ and $a_{\receiver} \in \mathcal{A}_{\receiver}$ while both being the state $s \in \mathcal{S}$. 
    %example
    In the Visual Discrimination Game, the reward could be the function equal to $1$ when the receiver picks up the correct image seen by the sender, $0$ otherwise.
    %
    %\item $\mathcal{I}:\{0,1\}\to [0,1]$ : is the probability that the sender and receiver perform an action at the current instance of the game. 
    %example
    %In the Visual Discrimination Game and more broadly in 2 players Lewis Games, there is an alternation between the sender action and the receiver action: first the sender sends a message, second the receiver tries to decode the message to achieve the task.
\end{itemize}

In Table~\ref{tab:taxo_tasks}, we show detail each of those elements for the most common examples used in machine learning simulations of language emergence.

\paragraph{The agents}

Lewis Games are decision making problems: the sender and receiver must agree on the best choice of actions in order to collect the maximum common reward. For instance, what combination of signals, namely what message, the sender must provide to let the receiver retrieve the correct image. The way the sender and receiver behave are characterized by action policies, i.e. decision-making rules:
\begin{itemize}
    \item $\pi_{\sender}$ is sender's policy, i.e. the message $m$ the sender sends when observing $o_{\sender}$. The policy $\pi_{\sender}$ is a probability distribution: $\pi_{\sender}(m|o_{\sender})$ is the probability of sending $m$ when observing $o_{\sender}$.
    % Language
    As described in Section~\ref{subsec:formalism_game}, the emergent language is the referential system that emerges between sender's views and the corresponding messages it sends. It means that the language is fully determined by sender's policy $\pi_{\sender}$ and that characterizing the emergent language is equivalent of characterizing $\pi_{\sender}$.
    
    % Visual discrimination game
    %In the Visual Discrimination Game, $\pi_{\sender}(m|o_{\sender})$ is the probability of sending $m$ when observing the image $o_{\sender}$.
    \item $\rho_{\receiver}$ is receiver's policy, i.e. the action $a_{\receiver}$ taken by the receiver when observing $o_{\receiver}$, its view of the state $s$ and sender's message $m$. The policy $\rho_{\receiver}$ is a probability distribution: $\rho_{\receiver}(a_{\receiver}|o_{\receiver})$ is the probability of picking action $a_{\receiver}$ when observing $o_{\receiver}$ (note that the sender's messages are included in the observation $o_{\receiver}$).
    % Visual discrimination game
    %In the Visual Discrimination Game, $\rho_{\reicever}(a_{\receiver}|o_{\receiver})$ is the probability of picking a given image when observing the set of all images (correct image and distractors) and sender's message.
\end{itemize}

In Section~\ref{subsec:design_agents}, we will show how those agents can be modelled as neural networks. 

\paragraph{The optimization problem}
Solving the game is an optimization problem: we aim at finding the best policies that will allow agents to maximize their common reward. In Section~\ref{subsec:design_optim}, we express this statement mathematically and use machine learning techniques to solve it. In communication games, note that language is viewed as a means of achieving communication, rather than having any other function. Consequently, there are two ways to evaluate the system: by assessing its performance on the task and by examining the characteristics of the language that emerges. We will discuss evaluation in more detail in Section \mathieu{XXX}.

\subsection{Framing communication games as a machine learning problem}
\label{subsec:comm_games_ML}

This section aims at showing how simulating language evolution can be framed as a machine learning problem. First, we briefly introduce machine learning and show how it applies to the simulation of language emergence and evolution in communication games (Sec~\ref{subsec:ML_comm}). We then restrict our scope to the study of Lewis Games~\citep{lewis1969convention}, a subclass of communication games, and state the machine learning problem in the context of those games (Sec.~\ref{subsec:lewis_games}). Eventually, we introduce a unified mathematical formalism to frame a Lewis Game as a machine learning problem (Sec.~\ref{subsec:formalism_game}).

\subsubsection{Machine learning is well suited for simulating communication games}
\label{subsec:ML_comm}

Over the past $50$ years, language evolution have largely been studied through communication games~\citep{lewis1969convention, steels1995self, baronchelli2010modeling}. As discussed in the Chapter \textit{Communication games: Modelling language evolution through dyadic interaction}, communication games are used to investigate how perceptual, interactive or environmental pressures shape the emergence of structure in communication protocols~\citep{kirby2008cumulative,cuskley2017regularity,raviv2019larger}.

During a communication game, participants build a language with the aim of achieving a given task. Language is learnt through trials and errors and a learning loop emerges between the participants. As such, when computationally modelling the game, machine learning is particularly suited to simulate this learning process. Indeed, machine learning can be defined as in~\cite{mitchell1997machine}:

\begin{displayquote}
        ``A computer program $f$ is said to learn from an experience $E$ with respect to some class of tasks $T$ and performance measure $P$, if its performance at tasks in $T$, as measured by $P$, improves with experience $E$.''
\end{displayquote}

In the context of a communication game, the participants are the computer programs $f$ which perform the communication task of the game $T$. After each instance of the game $E$, the success of the task is measured by $P$. The participants then improve by updating their communication protocol based of the outcome of their experience $E$. Optimally, if the process is repeated a sufficient number of times, the participants would \textit{converge}, i.e. stabilize on a successful communication protocol allowing them to solve the game. This learning loop is the fundamental idea of machine learning.

\subsubsection{Lewis Games: a standard communication game for machine learning}
\label{subsec:lewis_games}

\begin{figure}[ht!]
    \centering
    \includegraphics[width=\textwidth]{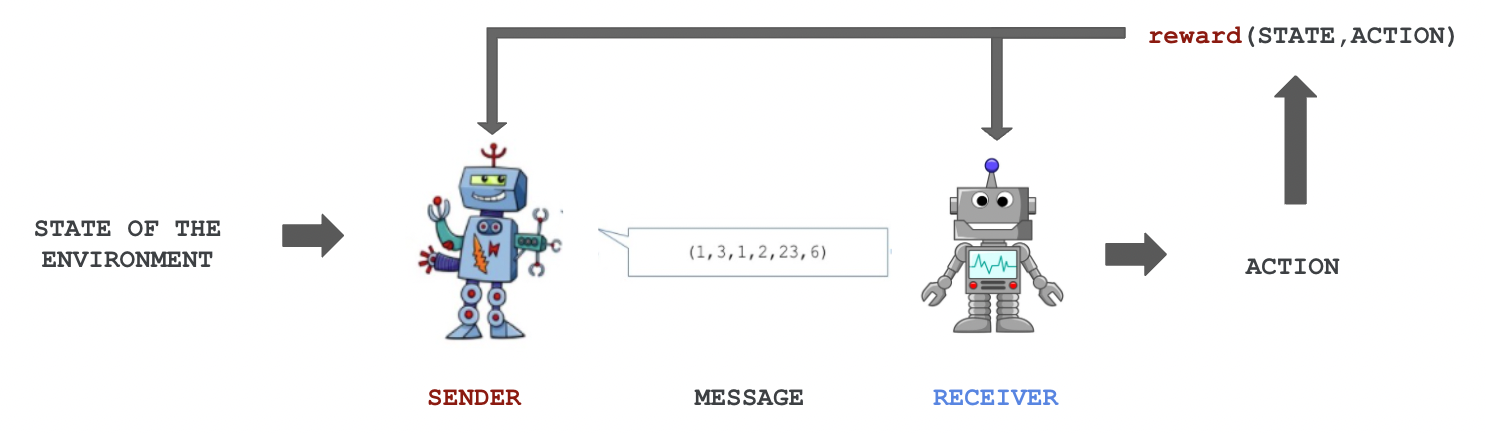}
    \caption{Scheme of the Lewis Game}
    \label{fig:scheme_lewis}
\end{figure}

Throughout this chapter, we will focus on a subclass of communication games as a guiding example: Lewis Games~\citep{lewis1969convention}. Historically, the emergence and evolution of signaling systems have extensively been studied through Lewis Games~\citep{lewis1969convention, skyrms2010signals} with recent applications in machine learning~\citep{lazaridou2020emergent}.
 In game theory, Lewis game are described as two-players cooperative games with incomplete information games~\citep{harsanyi1967games,kreps}, i.e. the two players have access to a different set of information, and have a perfect common interest to solve the game. In practice, Lewis Games proceed as follows:

\bigbreak  

Lewis signalling games involves two players: the sender and the receiver. Both players must solve a communication task in an environment. The environment is characterized at each time by a state. 
%While the sender has access to the state, the receiver cannot observe it. 
Agents do not have the same observations of the state and the receiver needs information from sender's view to achieve the task.
A play of the game is composed of the following steps:
\begin{itemize}
    \item The sender sends a message to the receiver to communicate about the state;
    \item The receiver chooses an action based on the message;
    \item Receiver's action gives rise to a reward that depends on the combination state-act. The reward is then cooperatively shared between the agents: the sender and receiver both receive the exact same reward for each play of the game.
\end{itemize}

In Table~\ref{tab:taxo_tasks}, we detail concrete examples of Lewis games that are commonly used when simulating language emergence and evolution in machine learning.

\begin{table}[ht!]
\begin{center}
\begin{tabular}{c c c c } 
 \hline
  Game & Task \\ [0.5ex] 
  \hline \hline
  Attribute reconstruction & The sender observes an image and send a message to describe it.  \\ [0.5ex] 
  Discrimination game & The receiver has to retrieve the image among a set of distractors.  \\ [0.5ex]
  Deal No-deal & dialogue-based, no embodiement  \\ [0.5ex]
  Instruction Following &  single/multi-turn, partial embodiement \\ [0.5ex]
  Color trails &  \\ full embodiement [0.5ex]
  &  \\
 \hline
\end{tabular}
\end{center}
\caption{Examples of variants of Lewis Games}
\label{tab:taxo_tasks}
\end{table}

Among the set of communication games, Lewis Games impose two additional assumptions: actions of the sender are restricted to sending messages and the reward is exactly the same for the two agents. As a results, the sender only aims at building a referential system between states and messages based on the feedback of the receiver: in other word, the sender must design a consistent communication protocol, and a fortiori, a language. 

When computationally simulating Lewis Games, each game can then be cast as the following machine learning problem:
\begin{displayquote}
        The \textbf{sender and receiver} ($f$) learn to maximize their common \textbf{reward} ($P$), i.e. the success of the \textbf{communication task} ($T$), based on \textbf{communicative interactions} ($E$). Language is the resulting referential system between sender's views and the corresponding messages it sends.
\end{displayquote}

%Taking \cite{mitchell1997machine}'s definition of machine learning, in a Lewis Game, the computer program $f=(f_{sender},f_{receiver})$ is the pair of communicative agents, the task $T$ is the task of the game, experiences $E$ are the successive play of the game and the performance $P$ is the common reward shared by the agents. In the following Section, we next aim at presenting, how all those elements should be modeled when designing a Lewis Game as a machine learning problem.
